# Supplementary material for: Ensemble Adversarial Training: Attacks and Defenses
Source: arXiv:1705.07204 source file (2020-04-26)
Supplement: Supplementary file 1 [file appendix-carlini.tex]

\section{Details for the $\ell_\infty$-Attack of Carlini and Wagner}
\label{apx:carlini}

We provide more details on the setup for the $\ell_\infty$-attack 
of Carlini and Wagner~\cite{carlini2016towards} evaluated in 
Section~\ref{sec:ensemble-training} for the MNIST models.
The original attack finds a perturbation $r$ by solving:\footnote{
We obtained better results by clipping the perturbed input to $[0,1]^d$, 
compared to using the change of variable suggested 
in~\cite{carlini2016towards}.
}
\[
\text{minimize}\quad c \cdot l(\min(\max(x+r, 0, 1))) + \sum_i \max( r_i - \tau, 0) \;.
\]
Here, $l(x')$ is some loss function (defined below), $c$ is a 
parameter weighting the two terms and $\tau$ is set so as to 
penalize large components of $r$.
For a data point $(x, y_{\text{true}})$, the loss function $l(x')$ is 
set to
\[
l(x') = \max\left(
	f(x)_{y_{\text{true}}} - \max\{f(x)_y : y \neq y_{\text{true}}\}
	, -\kappa \right) \;,
\]
where a large parameter $\kappa\geq 0$ favourizes
\emph{high-confidence} misclassifications.

When evaluating adversarially trained models in black-box settings, 
our goal is to produce adversarial examples that transfer with 
high probability. To craft 
perturbations that fool the source model with high confidence 
while satisfying the constraint $\norm{r}_\infty \leq \epsilon$,
we thus fix $\tau=\epsilon$ (we use $\epsilon=0.3$ in all our 
experiments). 
For all values of $\kappa \in \{1, 10, 20, 50, 100\}$, 
we perform a parameter search over $c$ by
iteratively solving the above optimization problem for increasingly 
large $c$ until the optimal solution violates the constraint 
$\norm{r}_\infty \leq \epsilon$.

This attack is much more computationally expensive than 
others we considered, including the iterative FGSM.
We apply the attack to the source model B for a subset of $1{,}000$ 
points from the MNIST test set. For $\kappa \geq 50$, model B 
misclassifies \emph{all} 
perturbed inputs with an average confidence of $99.5\%$. 
Transferring these adversarial examples yields error rates of 
$82.4\%$ on the undefended model A, $15.2\%$ on the adversarially 
trained model A$_\text{adv}$ and $7.0\%$ on our model A$_\text{adv-ens}$ 
using ensemble adversarial training.
The error rates are slightly higher than the ones obtained with 
the I-FGSM, although the difference is not statistically 
significant at $p=0.05$. To the best of our knowledge, it had not been 
previously observed that the I-FGSM and the above attack of Carlini 
and Wagner induce very similar error rates in black-box settings. 
Moreover, we see that when transferring examples to an adversarially 
trained model (whether using standard adversarial training or our 
ensemble variant), these iterative attacks perform only slightly 
better than the one-shot FGSM.
Thus, resource-constrained adversaries 
(e.g., those targeting \emph{real-time} or \emph{large-scale} evasion 
of a classifier) will have comparable success to attackers 
with more extensive resources (as required for the attack of Carlini 
and Wagner for instance).

Carlini and Wagner~\cite{carlini2016towards} found that computing the 
loss $l(x')$ above over the unnormalized logits, rather than using the 
cross-entropy loss as in the FGSM, leads to a stronger attack. 
It is possible that robustness to the above attack could be 
further improved by training on adversarial examples crafted with a 
variant of the FGSM where we compute the gradient at the logit layer.
