# Supplementary material for: Ensemble Adversarial Training: Attacks and Defenses
Source: arXiv:1705.07204 source file (2020-04-26)
Supplement: Supplementary file 2 [file appendix-failed-hypothesis.tex]

\section{Different Forms of Gradient Masking}
\label{ap:other-defenses}

If adversarial examples did not transfer, a natural defense against 
gradient-based attacks such as the FGSM could consist 
in hiding information about the model's gradient from the adversary.
For instance, if the model is non-differentiable (e.g, a Decision Tree) 
or if the model's gradient is zero at data points 
(i.e., the model is locally constant), gradient-based attacks are 
rendered ineffective. However, such defenses---referred to as 
``gradient masking'' mechanisms in~\cite{papernot2016towards}---are 
unlikely to prevent black-box attacks. Below, we review two different 
types of gradient masking, gradient \emph{hiding} and gradient 
\emph{smoothing} that affect potential defenses against adversarial 
examples. 

Given the prevalence of gradient masking in prior proposed defenses, 
we strongly encourage researchers to evaluate future defensive 
techniques in both white-box and black-box attack settings.

\paragraph{Gradient Hiding.}
Random Forests (RF) may seem ideal for preventing the 
attacks in Section~\ref{ssec:attacks}: the models are 
non-differentiable and highly non-linear.
Yet, RFs are easily fooled by 
transferring adversarial examples from a surrogate model: 
On MNIST, a RF of $100$ trees 
achieves $97.1\%$ accuracy on clean data, but FGSM 
examples ($\epsilon = 0.3$) crafted on a CNN transfer at a 
rate of $99\%$.
Defenses based on preventing an adversary from computing the 
gradient have also been proposed~\cite{wang2016using}. We 
conjecture that such methods are unlikely to provide robustness 
against black-box attacks.

\paragraph{Gradient Smoothing.}
Defensive distillation~\cite{papernot2016distillation} 
greatly reduces the effectiveness of white-box attacks 
by \emph{smoothing out} the model's gradient, leading to numerical 
instabilities in attacks such as the FGSM.
Yet, distilled models were shown to be evadable via 
black-box attacks where adversarial examples are transfered from 
undefended models~\cite{papernot2016practical}. Moreover, Carlini et 
al.~\cite{carlini2016towards} show successful white-box attacks 
with simple modifications of the FGSM attack~\cite{carlini2016towards}.  

The saturated networks from~\cite{nayebi2017biologically}
were found to perform a similar form of gradient 
masking~\cite{brendel2017comment} and are thus also likely vulnerable 
to black-box attacks.

\section{Other Hypotheses for Gradient Masking in Adversarial Training}
\label{ap:failed-hypotheses}

In Section~\ref{ssec:characterizing-grad-masking}, we show that 
adversarial training exhibits gradient masking by modifying the 
curvature of the model's loss function in the vicinity of data points.
Here, we discuss two alternative hypotheses we investigated, 
for explaining why adversarial 
training may lead to gradient masking: (1)
adversarial training \emph{smooths out} the models gradient, 
similarly to defensive distillation~\cite{papernot2016distillation};
 or (2) adversarial training overfits on the specific type of 
 adversarial examples encountered during training. 
However, we find neither of these hypotheses to be corroborated by our 
experiments.

\paragraph{Gradient Smoothing.}
Two proposed defenses against adversarial examples (Defensive 
Distillation~\cite{papernot2016distillation} and Saturated 
Networks~\cite{nayebi2017biologically}) hinder 
first-order attacks (in part) by rendering gradient computations 
numerically 
unstable~\cite{carlini2016towards, brendel2017comment}. These defenses 
can be evaded either through black-box 
attacks~\cite{papernot2016practical}, or via simple 
modifications to the FGSM to account for small gradient 
magnitudes~\cite{carlini2016towards, brendel2017comment}.

Previous work has established connections between adversarial 
training and a form of regularization of the model's 
gradient~\cite{goodfellow2014explaining, ororbia2017unifying}. 
Numerical instability 
of the gradient computation thus forms a natural hypothesis 
for the misleading robustness of adversarially trained models to 
white-box attacks. Yet, we find that adversarial training does not 
significantly smooth the gradient of the model's loss.

We compute the average gradient magnitude 
$\frac1n \sum_{i=1}^n \norm{\nabla_x J(x,y_{\text{true}})}_2$ over 
the full test set
for models B and B$_{\text{adv}}$ on MNIST, and the Inception v3 and 
v3$_{\text{adv}}$ models on ImageNet. The results appear in 
Table~\ref{table:grad-norms}. On MNIST, adversarial training has a 
minor regularization effect on the gradients. However, on ImageNet,
the average norm of the gradient \emph{increases} with 
adversarial training.

\begin{table}[h]
\caption{\textbf{Gradient norms with and 
without adversarial training.} Shows results on MNIST (left) and 
ImageNet (right) computed over the full test sets. \\[-0.5em]}
	\centering
	\begin{tabular}{@{}l c c @{\extracolsep{1cm}}c @{\extracolsep{10pt}}c@{}}
		 & \multicolumn{2}{c}{\textbf{MNIST}} & \multicolumn{2}{c}{\textbf{ImageNet}} \\
		%\cmidrule{2-3} \cmidrule{4-5}
		\textbf{Gradient Norm} & A & A$_{\text{adv}}$ & v3 & v3$_{\text{adv}}$ \\
		\toprule
		{mean} & $0.12$ & $0.11$ & $0.10$ & $0.17$  \\
		{stdev} & $0.95$ & $0.81$ & $0.15$ & $0.23$\\
		\bottomrule
	\end{tabular}
	\label{table:grad-norms}
\end{table}

\paragraph{Overfitting.}

Adversarial training using a particular 
attack technique (e.g., FGSM) typically fails to significantly 
increase robustness to other attacks  (e.g., iterative 
strategies)~\cite{kurakin2016scale}.\footnote{
	Kurakin et al.~\cite{kurakin2016scale} note that iterative attacks 
	tend to transfer at a much lower rate compared to non-iterative 
	attacks. Thus, even if adversarial training does not substantially 
	increase robustness to iterative attacks, the model may still be 
	secure against black-box attacks.} 
Another hypothesis to explain gradient masking
when models are adversarially trained is that the defense
``overfits'' to the particular attack directions computed from the 
trained model. In other words, maybe the number of different 
adversarial perturbations is so large, that adversarial training 
successfully increases the model's margins in adversarial directions 
that it sees (i.e., the ones given by the model's gradient at 
each training point), but remains vulnerable to other 
unseen perturbations.

However, the overfitting hypothesis also fails to appropriately 
explain the vulnerability of adversarial training to 
black-box attacks. Indeed, even non-defended 
models tend to have large margins in the ``adversarial'' directions 
computed on the adversarially trained models. The results in
Table~\ref{table:black-box} show that FGSM samples 
crafted on the adversarially trained models are easier to classify 
for all models. Thus, as argued in 
Section~\ref{ssec:characterizing-grad-masking}, it appears that 
adversarial training leads to models for which the FGSM mostly 
produces ``easy'' perturbations, although there exist other 
vulnerable directions.
